# Supplementary material for: A 2-3 mm high-resolution molecular line survey towards the centre of the nearby spiral galaxy NGC 6946
Source: arXiv:2201.02209 source file (2022-01-10)
Supplement: Supplementary file 1 [file CO10.tex]

\begin{figure*}
    \centering
    \includegraphics[width=1.0\textwidth]{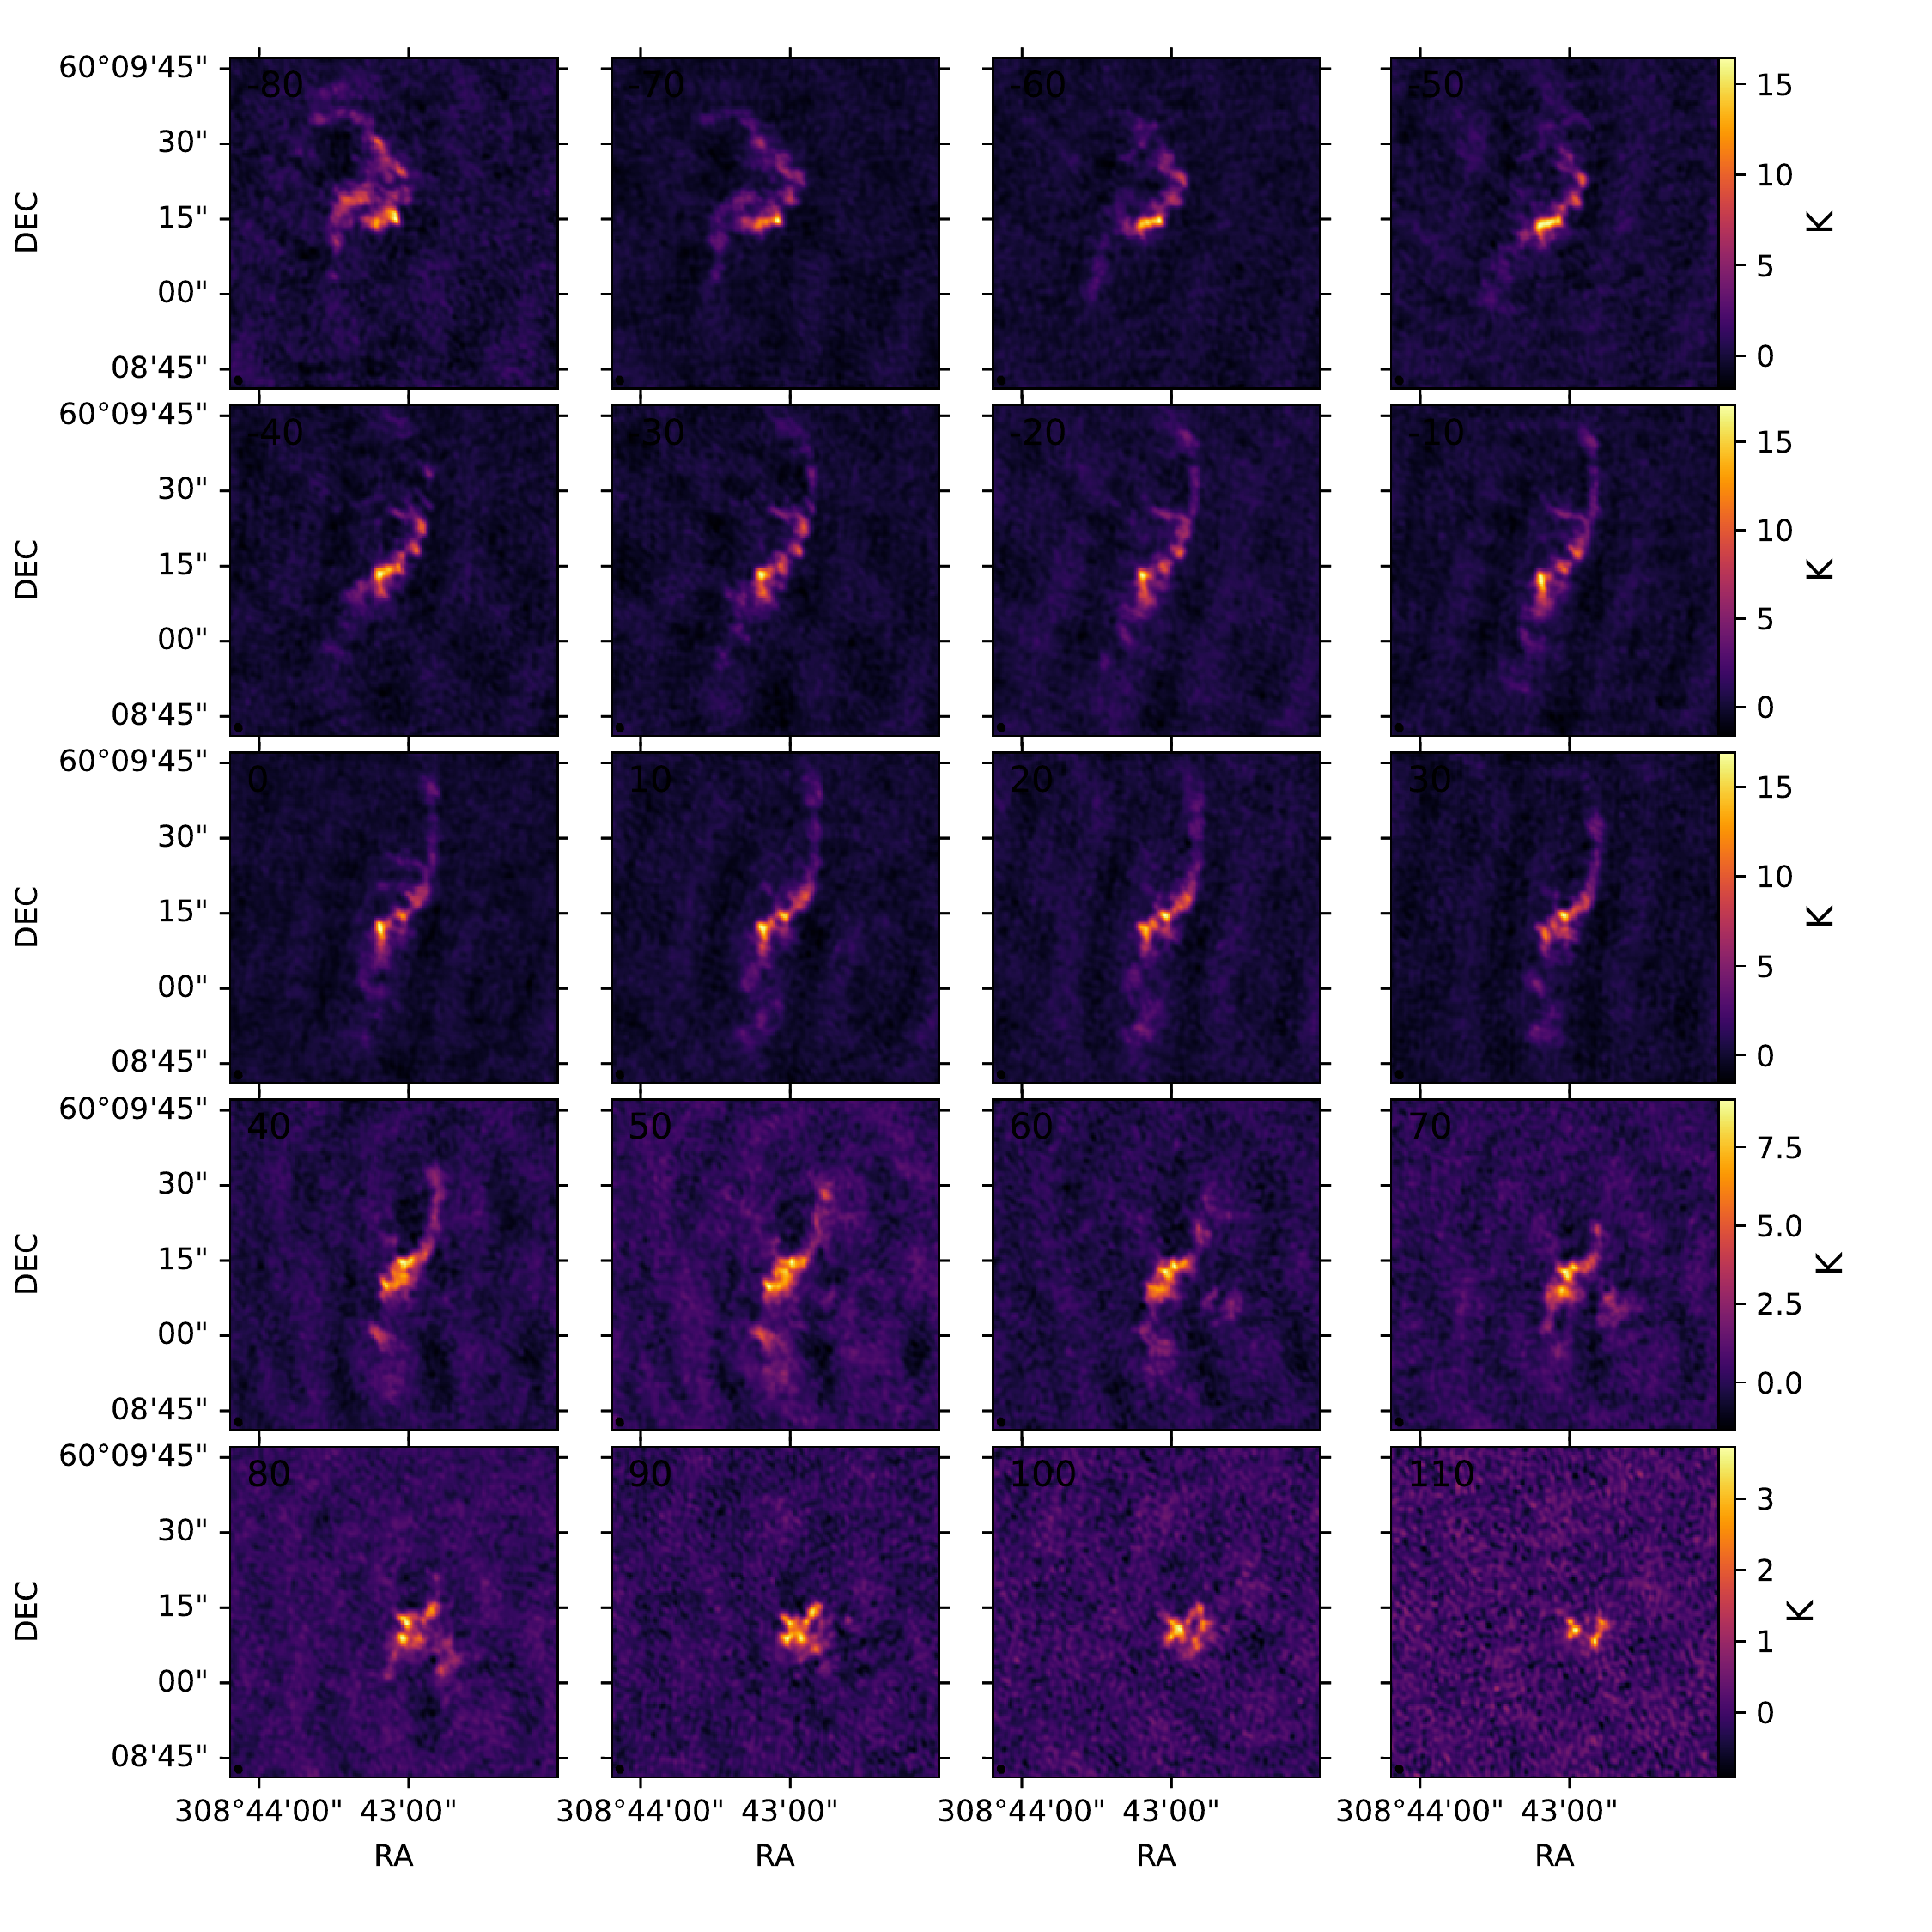}
    
    \caption{CO(1-0) channel maps, from -80 to 110 km s$^{-1}$.}
    \label{app:channelmap_first}
\end{figure*}
